# Supplementary material for: Azimuthal correlations in photoproduction and deep inelastic $\boldsymbol{ep}$ scattering at HERA
Source: arXiv:2106.12377 ancillary file (2022-05-22)
Supplement: Supplementary file 1 [file AdditionalMaterial.pdf]

# Azimuthal correlations in photoproduction and deep inelastic *ep* scattering at HERA

**Additional material**

ZEUS Collaboration

## 1 PYTHIA 8.303 settings

The ZEUS photoproduction data is compared to Monte Carlo events generated using PYTHIA 8.303 in the article. The main parameter of interest in this analysis is  $p_{T0}^{\text{ref}}$ , which controls the amount of Multiparton Interactions (MPI). The PYTHIA settings used are shown in Table 1.

| Setting type                   | choice(s)                                |
|--------------------------------|------------------------------------------|
| Beams:frameType                | 2 (CM)                                   |
| Beams:eA                       | 920 GeV                                  |
| Beams:eB                       | 27.52 GeV                                |
| Beams:idA                      | 2212                                     |
| Beams:idB                      | 11                                       |
| PDF:lepton2gamma               | on (enables photon sub-beam from lepton) |
| Photon:Q2max                   | 1.0 GeV <sup>2</sup>                     |
| Photon:Wmin                    | 10 GeV                                   |
| Photon:ProcessType             | 0 (auto mix of resolved and direct)      |
| PhotonParton:all               | on (direct component)                    |
| SoftQCD:nonDiffractive         | on (resolved component)                  |
| PartonLevel:MPI                | on or off (master switch for MPI)        |
| MultipartonInteractions:pT0Ref | 2, 3, 4 GeV (MPI strength)               |
| ColourReconnection:range       | 0.0, 1.8 (range in p-space of CR)        |

Table 1: PYTHIA 8.303 settings used to generate photoproduction MC data.

Generated charged particles were retained if they satisfy the definition of primary particles listed in the main article. About 10 M events with  $N_{\text{ch}} \geq 20$  were generated for each variation.

## 2 PYTHIA 6.220 comparisons

Tracking efficiency and trigger-bias corrections for the results in the main article were obtained from existing PYTHIA 6.220 photoproduction Monte Carlo with the ZEUS detector simulation. The Monte Carlo data was generated with a jet preselection of at least one jet per event. Massless jets were reconstructed with the  $p_T$ -recombination scheme using final-state hadrons with  $E_T > 3$  GeV and  $|y| < 3$ .

### 3 Supplementary figures

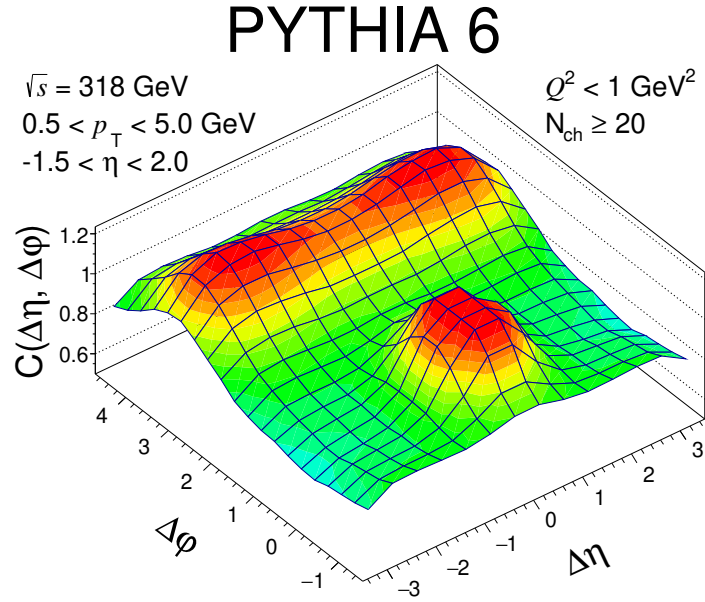

Figure 1: Reconstructed two-particle correlations,  $C(\Delta\eta, \Delta\phi)$ , in PYTHIA 6.220 photoproduction Monte Carlo. The plot was symmetrised along  $\Delta\eta$ .

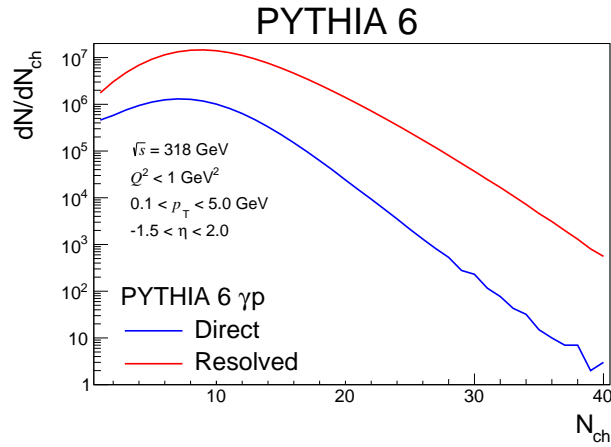

Figure 2: Generator-level distributions of charged particles for the resolved and direct photoproduction components of PYTHIA 6.220 Monte Carlo.

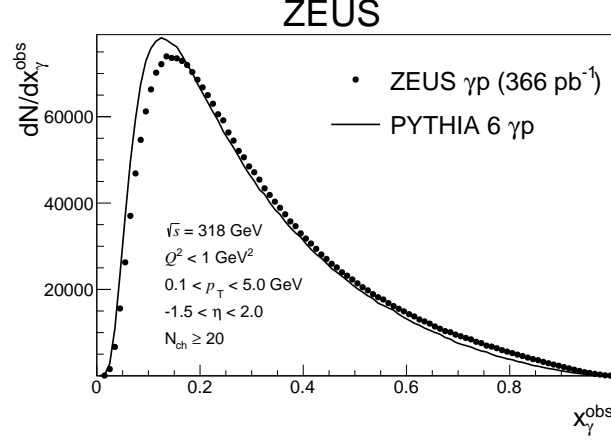

Figure 3: Reconstructed  $x_\gamma^{\text{obs}}$  distribution in ZEUS photoproduction data compared to PYTHIA 6.220 Monte Carlo in events with at least 2 jets. The  $x_\gamma^{\text{obs}}$  distribution was reconstructed using the two leading jets and represents the fraction of the exchanged-photon energy and longitudinal momentum that is transferred to the observed particle production in the two jets and is given by  $(E^{\text{jet},1} + E^{\text{jet},2} - p_Z^{\text{jet},1} - p_Z^{\text{jet},2})/(E^{\text{all}} - p_Z^{\text{all}})$ . Massive jets were reconstructed with the E-scheme and in inclusive mode. Dead material corrections were applied. Jets were required to have transverse energy greater than 2.5 GeV and pseudorapidity from -2.5 to 2.5.

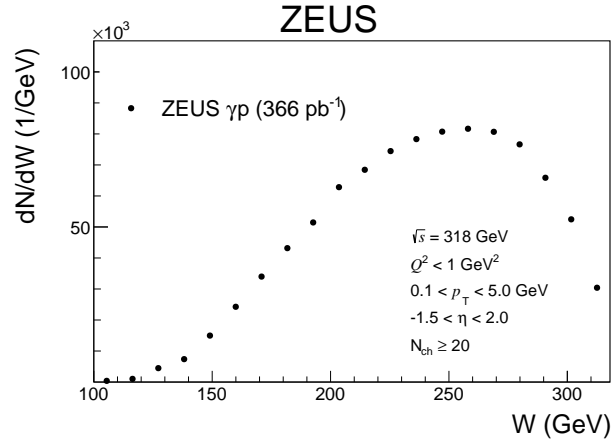

Figure 4: Reconstructed  $W$  distribution in ZEUS photoproduction data, where  $W = \sqrt{2 E_p (E - p_Z)}$ , which corresponds to the  $\gamma p$  centre-of-mass energy. The  $E - p_Z$  was measured using ZEUS final-state energy-flow objects. The mean and RMS of this  $W$  distribution is 239 and 43 GeV, respectively.

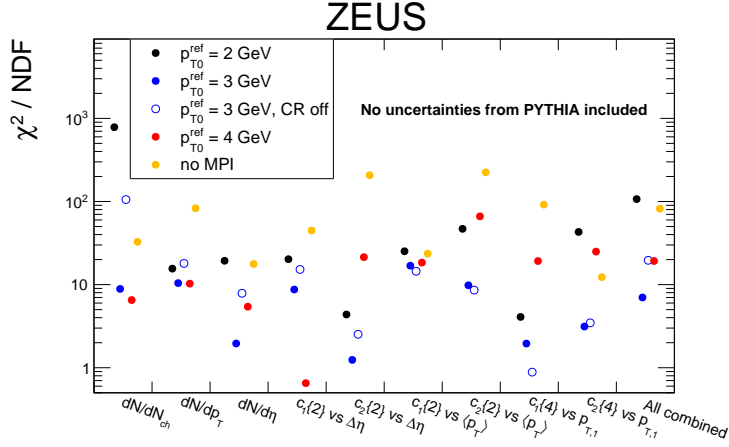

Figure 5: Compressed overview of the comparison between ZEUS photoproduction data and PYTHIA 8 predictions. The  $\chi^2$  is computed using the combined statistical and systematic uncertainties of ZEUS data. No uncertainties from PYTHIA predictions were included. The type of observable is shown on the x-axis.

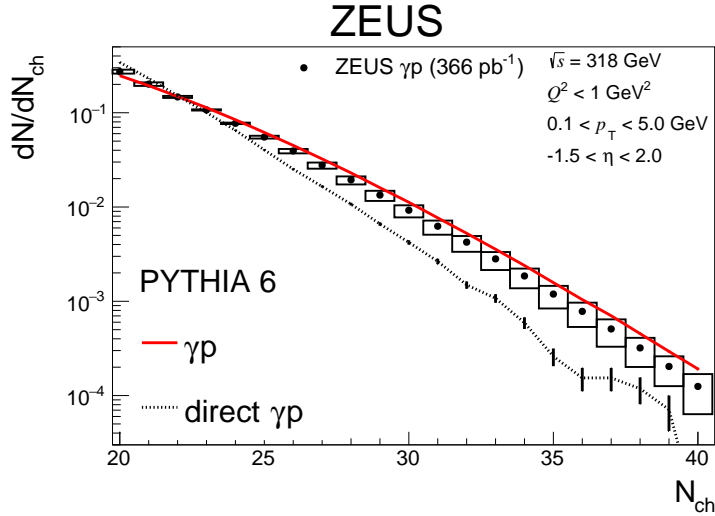

Figure 6: Charged-particle multiplicity distribution  $dN/dN_{\text{ch}}$  compared to PYTHIA 6.220 photoproduction Monte Carlo. The direct and total (resolved + direct)  $\gamma p$  processes are shown. The lines connect the central values of the Monte Carlo points. The integral of the distributions in the range shown is normalised to unity. The statistical uncertainties are shown as vertical lines although they are typically smaller than the marker size. Systematic uncertainties are shown as boxes around the data points.

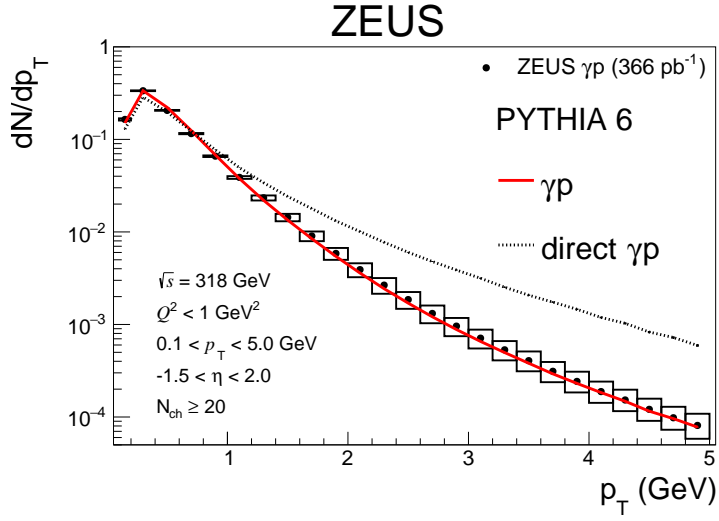

Figure 7: Charged-particle transverse momentum distribution  $dN/dp_T$ . Other details as in Fig. 6.

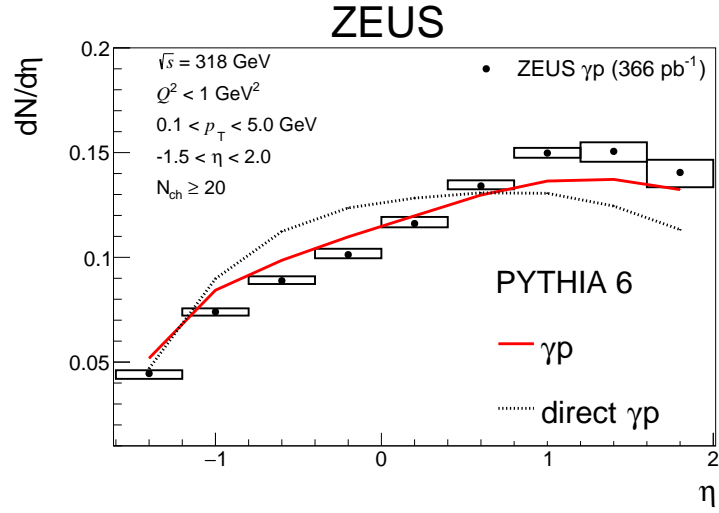

Figure 8: Charged-particle pseudorapidity distribution  $dN/d\eta$ . Other details as in Fig. 6.

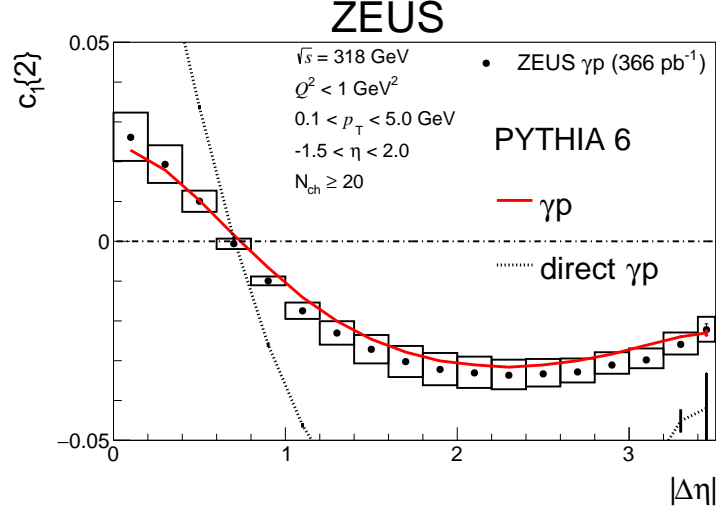

Figure 9: Two-particle azimuthal correlations  $c_1\{2\}$  versus  $|\Delta\eta|$  compared to PYTHIA 6.220 photoproduction Monte Carlo. The direct and total (resolved + direct)  $\gamma p$  processes are shown. The lines connect the central values of the Monte Carlo points. The statistical uncertainties are shown as vertical lines although they are typically smaller than the marker size. Systematic uncertainties are shown as boxes around the data points.

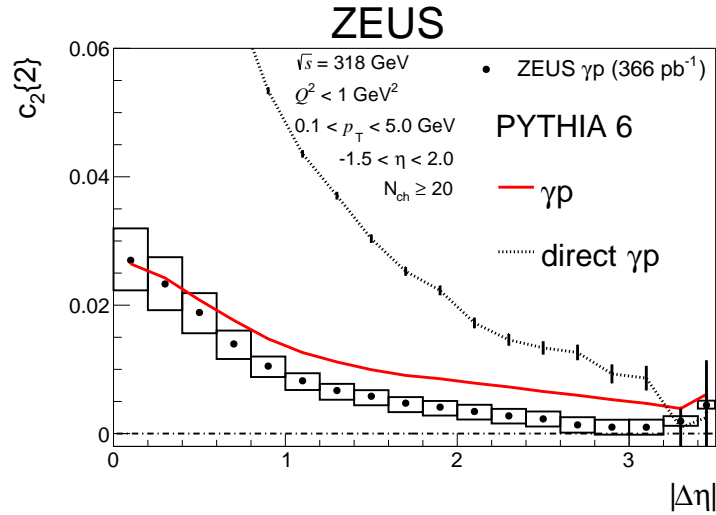

Figure 10: Two-particle azimuthal correlations  $c_2\{2\}$  versus  $|\Delta\eta|$ . Other details as in Fig. 9.

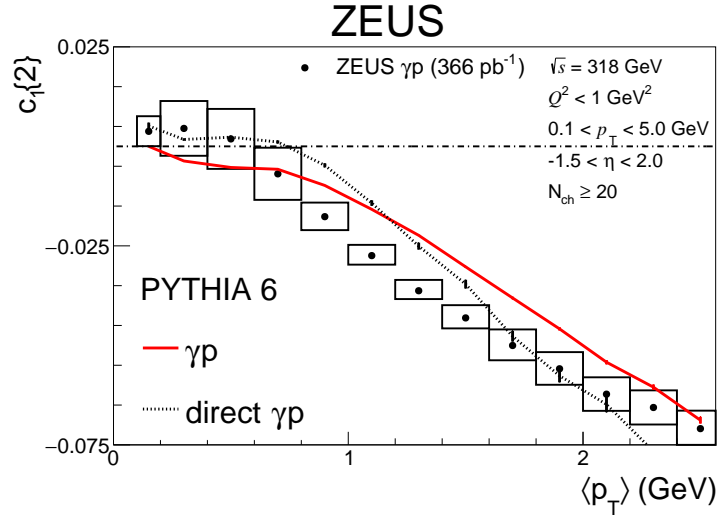

Figure 11: Two-particle azimuthal correlations  $c_1\{2\}$  versus  $\langle p_T \rangle$ . Other details as in Fig. 9.

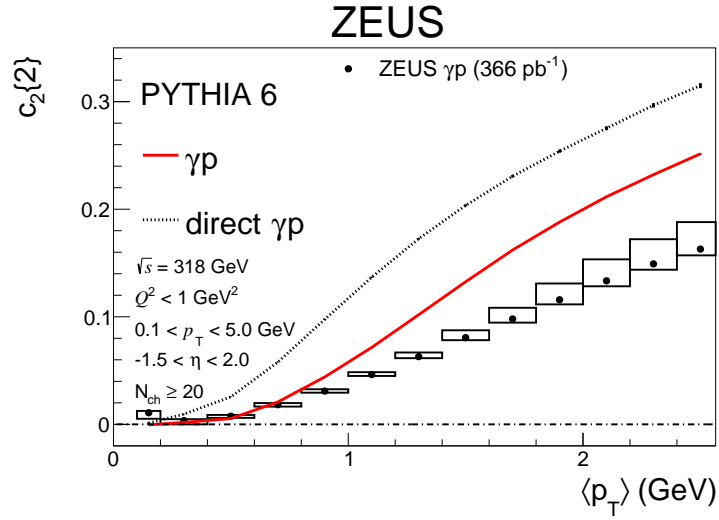

Figure 12: Two-particle azimuthal correlations  $c_2\{2\}$  versus  $\langle p_T \rangle$ . Other details as in Fig. 9.

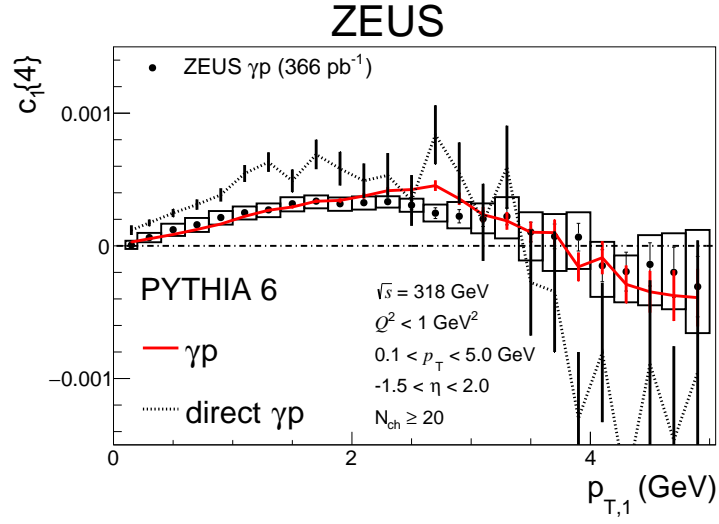

Figure 13: Four-particle azimuthal correlations  $c_1\{4\}$  versus  $p_{T,1}$ . Other details as in Fig. 9.

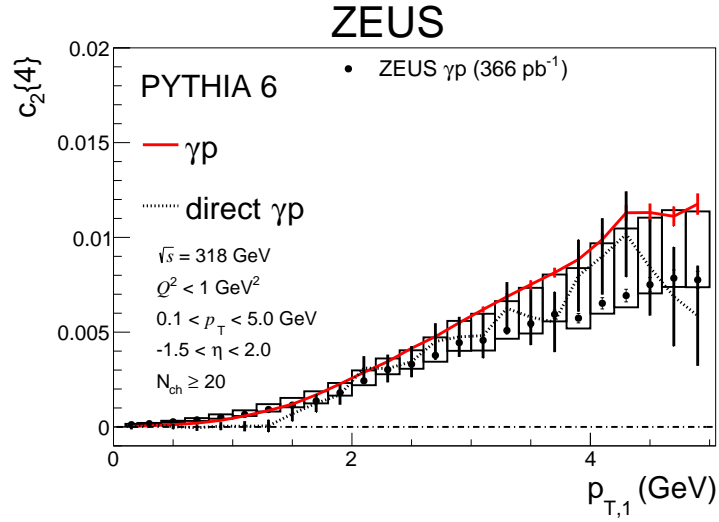

Figure 14: Four-particle azimuthal correlations  $c_2\{4\}$  versus  $p_{T,1}$ . Other details as in Fig. 9.
